# Supplementary material for: Nonlinear differential equations on non-compact domains
Source: arXiv:math/0210142 source file (2002-10-16)
Supplement: Supplementary file 1 [file partappendix.tex]

\part{Appendix}
